# Supplementary material for: Spin structure of K valleys in single-layer WS$_2$ on Au(111)
Source: arXiv:1807.11235 source file (2018-10-01)
Supplement: Supplementary file 1 [file Supplement_WS2_Paper_2018-08-31.pdf]

# Supplement to "Spin structure of K valleys in single-layer WS<sub>2</sub> on Au(111)"

Philipp Eickholt,<sup>1</sup> Charlotte Sanders,<sup>2</sup> Maciej Dendzik,<sup>2</sup> Luca Bignardi,<sup>3</sup> Daniel Lizzit,<sup>3</sup> Silvano Lizzit,<sup>3</sup> Albert Bruix,<sup>2</sup> Philip Hofmann,<sup>2</sup> and Markus Donath<sup>1</sup>

<sup>1</sup>*Physikalisches Institut, Westfälische Wilhelms-Universität Münster,  
Wilhelm-Klemm-Straße 10, 48149 Münster, Germany*

<sup>2</sup>*Department of Physics and Astronomy, Interdisciplinary Nanoscience  
Center (iNANO), Aarhus University, 8000 Aarhus C, Denmark*

<sup>3</sup>*Elettra-Sincrotrone Trieste ScPA, Trieste 34149, Italy*

## I. DETAILS OF THE FITTING PROCEDURE TO EXTRACT PEAK POSITIONS

To extract the spin-dependent peak positions and the resulting spin splittings, we fitted the individual spin spectra separately. The spectra for  $\theta \geq 65^\circ$  in Fig. 2 of the main paper show one dominant spectral feature on an almost linearly increasing background. Therefore, our fit functions  $F$  consist of a Lorentzian function  $L$  on a background  $B$ , multiplied by the Fermi distribution  $f$  at room temperature for unoccupied states. The result is then convoluted with the apparatus function  $A$ , which is approximated by a Gaussian function with full width at half maximum (FWHM) of 350 meV<sup>1</sup>.

$$F = A * [f(L + B)] \quad (1)$$

The background  $B$  consists of a spin-independent constant part due to dark counts of the photon detectors plus an energy- and spin-dependent part due to secondary processes, mainly caused by electron scattering creating an electron-hole-pair preceding the optical transition. The exact shape of the latter part of the background intensity is difficult to model. A simple approach assumes random  $\mathbf{k}$  approximation and constant transition probabilities in the case of angle-integrated measurements, which leads to model calculations based on the density of states<sup>2</sup> (see also model calculations in Ref. 3). In our case of  $\mathbf{k}$ -resolved measurements, however, the random  $\mathbf{k}$  approximation has to be questioned. Obviously, the linear background above the peak energy is higher than the extrapolation of the linear background below the peak energy. This reflects the increase of the density of states at the conduction-band minimum of WS<sub>2</sub>. Therefore, we modeled this background increase by a step function at the position of the dominating spectral feature. Figure 1 presents the individual components for the fitting procedure to extract the peak positions in Fig. 4 of the main paper: Lorentzian function  $L$ , linear background (spin-independent slope) with a spin-dependent step-like increase at the position of  $L$  (model A). Both components are added and multiplied with the Fermi distribution  $f$ . The result is then convoluted with the apparatus function  $A$  resulting in the solid lines through the data points.

The fits show good agreement with the data except for a systematic deviation in the energy region around the Fermi energy. Here, the spectra are influenced by the

density of states of the Au substrate, which results in a different slope of the background compared with the slope at higher energies. Note that our inverse-photoemission data of bulk WS<sub>2</sub> samples (not shown) do not exhibit this intensity at the Fermi level. We decided not to include additional functions (and fitting parameters) in the fitting procedure to model this substrate-induced intensity because the peak position of  $L$  is energetically well separated, and additional fitting parameters don't make the fitting more conclusive.

To evaluate the statistical relevance of the result, a fitting program provides usually uncertainty intervals for the best fitting parameters, based on the statistical uncertainties of the data points  $n_{\uparrow,\downarrow}$ , which in a counting experiment is given by  $\sqrt{n_{\uparrow,\downarrow}}$ . [The statistical uncertainties of  $N_{\uparrow,\downarrow}$ , the counts for a hypothetically 100% spin-polarized electron beam, are derived using Eq. 6 (see Sect. 2) by propagation of uncertainties.] An equivalent way to derive the statistical uncertainties of the fitting parameters, which is more intuitive and illustrative, was used in former publications<sup>3-5</sup>. Pseudospectra are produced by varying each data point randomly according to its own statistical uncertainty. Each pseudospectrum is fitted with the described fitting functions and the obtained peak positions are collected in a histogram. The histogram showing the peak position distribution  $N(E)dE$  is a direct measure of the most probable peak position and its uncertainty. These distributions are displayed in the lower panels of Fig. 4 of the main paper.

To test the stability and reliability of the fitting routine, we modified the fitting parameters in the following way:

- Model B: One might argue that the step-like background increase due to the onset of the density of states at the conduction-band minimum is better described by an integral over the peak  $L$ . Therefore, we also tried a broadened step function to account for that.
- Model C: It is reasonable to assume the energy position of the step function to be spin dependent because the conduction-band minimum is spin dependent. However, we also tested a spin-independent position of the step-like background increase.
- Model D: In addition, we tested the influence of the energy position of the step function. We shifted

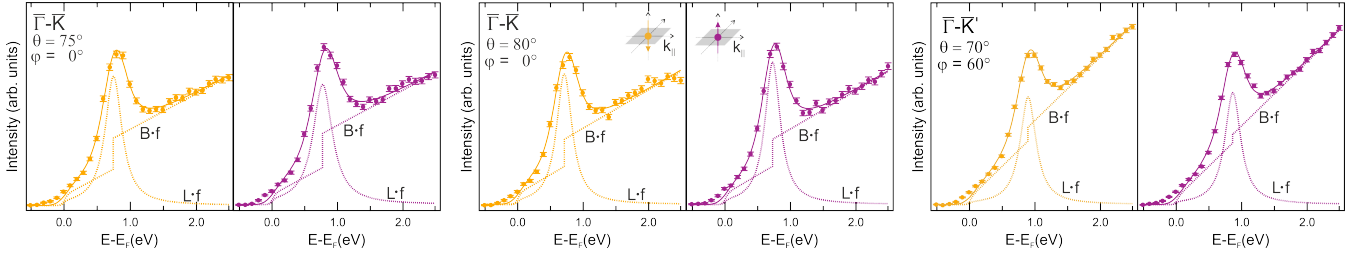

FIG. 1. Spin-resolved inverse photoemission spectra of Fig. 4 of the main paper together with their fit components:  $B \cdot f$  ( $L \cdot f$ ) denotes the background (Lorentzian function) multiplied by the Fermi distribution. The background consists of a linear function with a step function at the position of  $L$  (see text for details).

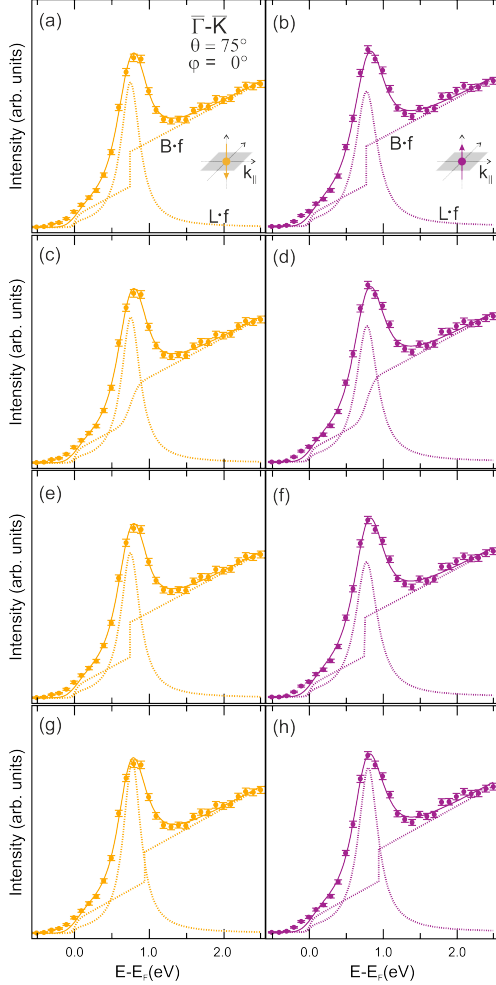

FIG. 2. Test of reliability and stability of the fitting routine for the spectra of  $\theta = 75^\circ$  along  $\bar{\Gamma} - \bar{K}$ : (a,b) model A as used in Fig. 1, (c,d) model B [broadened step function], (e,f) model C [spin-independent step energy], and (g,h) model D [spin-independent step energy, shifted by 0.2 eV to higher energy with respect to  $L$ ].

the step function to 0.2 eV higher energy for both individual spin spectra.

Figure 2 provides an example of the described tests

for one data set ( $\theta = 75^\circ$  along  $\bar{\Gamma} - \bar{K}$ ). Table I presents the obtained peak positions and corresponding spin splittings. While the different models result in slightly different absolute peak positions, the spin splittings are reliable within the uncertainty intervals.

TABLE I. Test of stability and reliability of the fitting routine. Spin-dependent energy positions of  $L$  and spin splittings for models A, B, C, and D for one data set ( $\theta = 75^\circ$   $\bar{\Gamma} - \bar{K}$ ).

| Fit model | $E_\uparrow$ (meV) | $E_\downarrow$ (meV) | $\Delta E_{\uparrow\downarrow}$ (meV) |
|-----------|--------------------|----------------------|---------------------------------------|
| Model A   | 773.4              | 747.5                | 25.9                                  |
| Model B   | 779.6              | 753.3                | 26.3                                  |
| Model C   | 773.3              | 747.5                | 25.8                                  |
| Model D   | 793.5              | 770.6                | 22.8                                  |

Based on the spin-resolved photoemission results, which showed completely spin-polarized states, we had reasonably assumed that the same is true for the states at the conduction-band minimum. Nevertheless, we considered that the states are not completely spin polarized, i.e., each individual spin spectrum consists of a two-peak structure with different intensities for the two peaks. For an assumed spin polarization of 80% instead of 100% in both conduction bands, the two peaks would have an intensity ratio of 9:1. While it is not possible to use the peak splitting as a free parameter in the fitting routine due to the overlapping states, one can estimate the outcome. Fitting the peak with two Lorentzians, e.g., a dominant part at lower energy and a minor part at higher energy in one individual spin spectrum, shifts the peak energy of the dominant part to lower energy compared with the fit with only one Lorentzian. Vice versa, in the other individual spin spectrum, the peak energy of the dominant part is shifted to higher energy. As a consequence, the derived spin splitting will be larger if the spin polarization of the conduction band is not 100%. In addition, we tried to fit the data with a given but variable peak splitting for both individual spin spectra. The result was consistent with the expectation: The energy difference between the dominating peaks in the two individual spin spectra was slightly larger ( $\approx 3$  meV, data for  $\theta = 80^\circ$ ) than the spin splittings obtained from

a fit with one Lorentzian function. In conclusion, the spin splittings derived from a fit with one Lorentzian is a lower limit as stated in the main paper. Any reasonable assumption of the conduction-band spin polarization will only slightly enhance the spin splitting.

## II. OBTAINING INDIVIDUAL SPIN SPECTRA FROM RAW (INVERSE) PHOTOEMISSION DATA

This section provides a short tutorial of how to derive individual spin spectra from raw photoemission and inverse photoemission data, which are obtained with non-ideal spin-polarization detectors and spin-polarized electron sources, respectively.

Angle-resolved photoemission and inverse photoemission are the two most direct techniques to determine the occupied and unoccupied electronic states of solid surfaces. Adding spin resolution offers access to the spin character of the investigated bands. In photoemission, a spin-polarization detector has to be used after the photoelectrons have passed an energy analyzer. To detect the spin character, different types of detectors are applied, either based on exchange or on spin-orbit interaction. Using exchange interaction in ferromagnetic scattering targets, the scattered intensity from a ferromagnetic film depends on the magnetization of the target [very low-energy electron diffraction (VLEED) detector]. Two measurements on the oppositely magnetized target (**M** and **-M**) yield an asymmetry  $A = (n_{\mathbf{M}} - n_{-\mathbf{M}})/(n_{\mathbf{M}} + n_{-\mathbf{M}})$ . Using high-energy scattering [Mott detector] or low-energy scattering [spin-polarized low-energy electron diffraction (SPLEED) detector] on a high- $Z$  material, a left-right asymmetry  $A = (n_l - n_r)/(n_l + n_r)$  of the scattering is observed, caused by spin-orbit interaction.

In both cases, the obtained asymmetry reflects the spin polarization of the scattered electrons. The spin separation is, however, not complete. The spin-resolving power of the detector is characterized by the so-called Sherman function  $S$ , defined by the scattering asymmetry  $A$  for a 100% polarized electron beam.  $S$  depends on the type of detector, the experimental parameters, and the target condition, ranging from a few percent to some tens of percent. Provided the Sherman function  $S$  of a detector is known from an independent calibration measurement (in our case 24%), the spin polarization of the emitted photoelectrons  $P = (N_{\uparrow} - N_{\downarrow})/(N_{\uparrow} + N_{\downarrow})$  is given by

$$P = \frac{A}{S}. \quad (2)$$

The individual or sometimes called partial spin-up and spin-down data  $N_{\uparrow}$  and  $N_{\downarrow}$  are obtained from the polarization  $P$  and the total number of electrons  $N = n_{\mathbf{M}} + n_{-\mathbf{M}}$  or  $N = n_l + n_r$  by

$$N_{\uparrow} = \frac{N}{2}(1 + P) = \frac{N}{2}\left(1 + \frac{A}{S}\right) \quad (3)$$

and

$$N_{\downarrow} = \frac{N}{2}(1 - P) = \frac{N}{2}\left(1 - \frac{A}{S}\right) \quad (4)$$

with  $N = n_{\mathbf{M}} + n_{-\mathbf{M}} = N_{\mathbf{M}} + N_{-\mathbf{M}}$  or  $N = n_l + n_r = N_l + N_r$ .  $n$  denotes the number of electrons measured with the non-ideal spin-polarization detector,  $N$  the number of electrons measured with an hypothetically ideal spin-polarization detector. In the case of different sensitivities of the electron detectors for left and right scattering, additional apparatus asymmetries appear that have to be taken care of. Detailed descriptions about the described issues are found in the literature, see, e.g.<sup>6-8</sup>.

In inverse photoemission, spin resolution is achieved by using a spin-polarized electron beam. However, the spin polarization  $P$  of the electron beam is not 100%, in our case  $P = 29\%$ . The incomplete spin polarization of the electron beam in inverse photoemission plays the same role as the incomplete spin separation of the spin-polarization detector in photoemission. Therefore, to obtain the individual spin spectra, the equivalent procedure as in photoemission has to be applied.  $P$  has to be known from an independent calibration measurement. Here,  $n_{\uparrow, \downarrow}$  denote the number of photons detected for the two opposite spin polarization directions of the electron beam. The observed asymmetry in the number of photons  $A = (n_{\uparrow} - n_{\downarrow})/(n_{\uparrow} + n_{\downarrow})$  is smaller than the asymmetry for a hypothetically 100% spin-polarized beam  $A/P = (N_{\uparrow} - N_{\downarrow})/(N_{\uparrow} + N_{\downarrow})$ . The individual spin spectra are obtained from the beam spin polarization  $P$  and the total number of photons  $N = N_{\uparrow} + N_{\downarrow} = n_{\uparrow} + n_{\downarrow}$  by

$$N_{\uparrow, \downarrow} = \frac{N}{2}\left(1 \pm \frac{A}{P}\right). \quad (5)$$

In the case of non-collinearity between the spin-quantization axes of sample and spin-polarization detector or electron source, this angle has to be taken into account. In our case, the spin-quantization axis at  $\bar{K}$  and

TABLE II. Influence of the assumed spin polarization  $P$  of the incoming electrons.

|                                           | $E_{\uparrow}$ (meV) | $E_{\downarrow}$ (meV) | $\Delta E_{\uparrow\downarrow}$ (meV) |
|-------------------------------------------|----------------------|------------------------|---------------------------------------|
| $\theta = 80^\circ \bar{\Gamma}-\bar{K}$  |                      |                        |                                       |
| Raw data                                  | $722.3 \pm 2.0$      | $717.8 \pm 2.0$        | $4.5 \pm 2.8$                         |
| Data for $P = 32\%$                       | $726.9 \pm 4.5$      | $712.4 \pm 5.0$        | $14.5 \pm 6.8$                        |
| Data for $P = 29\%$                       | $727.5 \pm 4.9$      | $711.5 \pm 5.4$        | $16.0 \pm 7.4$                        |
| Data for $P = 26\%$                       | $728.4 \pm 5.4$      | $710.5 \pm 6.1$        | $17.9 \pm 8.2$                        |
| $\theta = 70^\circ \bar{\Gamma}-\bar{K}'$ |                      |                        |                                       |
| Raw data                                  | $875.1 \pm 1.7$      | $884.3 \pm 1.8$        | $-9.2 \pm 2.4$                        |
| Data for $P = 32\%$                       | $865.8 \pm 3.9$      | $893.8 \pm 3.9$        | $-28.0 \pm 5.5$                       |
| Data for $P = 29\%$                       | $864.5 \pm 4.3$      | $895.3 \pm 4.3$        | $-30.8 \pm 6.1$                       |
| Data for $P = 26\%$                       | $862.9 \pm 4.7$      | $897.1 \pm 4.8$        | $-34.3 \pm 6.7$                       |

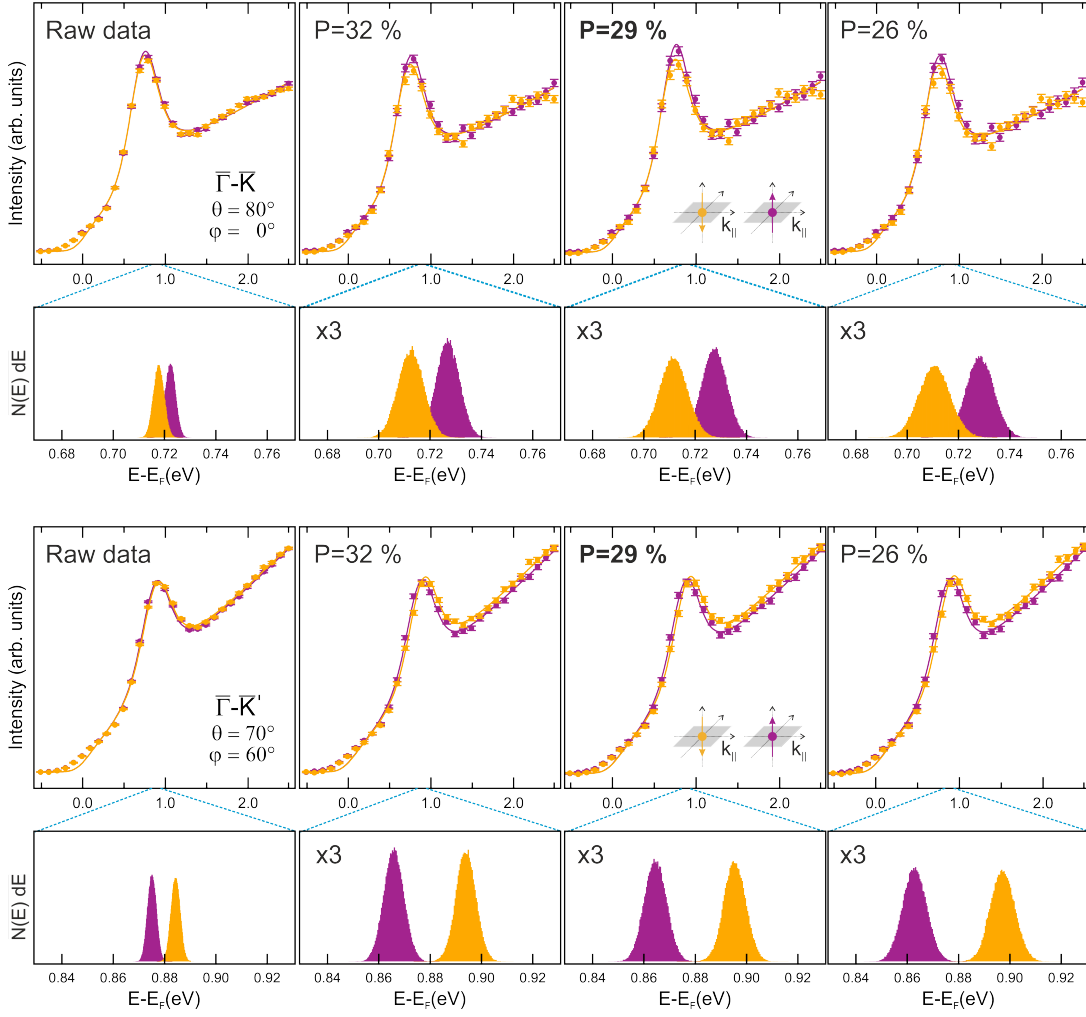

FIG. 3. Inverse photoemission spectra for  $\theta = 80^\circ$  along  $\bar{\Gamma} - \bar{K}$  (upper panel) and for  $\theta = 70^\circ$  along  $\bar{\Gamma} - \bar{K}'$  (lower panel). From left to right: Raw data and spin-resolved data normalized to 32, 29, and 26% spin polarization of the electron beam together with corresponding peak-position distributions  $N(E)dE$ .

$\bar{K}'$  is out of plane and the electron beam is transversally spin polarized. As a consequence, the spin sensitivity is zero for normal electron incidence and increases with increasing angle of incidence  $\theta$ , as it was discussed in the case of Tl/Si(111), see Ref. 9. Equation 4 modifies to

$$N_{\uparrow,\downarrow} = \frac{N}{2} \left( 1 \pm \frac{A}{P \sin \theta} \right). \quad (6)$$

For a more detailed description of this "normalization" procedure in inverse photoemission, the reader is referred to the literature<sup>1,10,11</sup>.

An important input to determine the individual spin spectra measured with nonideal spin-polarization detectors and electron sources is the exact knowledge of  $S$

and  $P$ , respectively. Any uncertainty of  $S$  and  $P$  influences the outcome of the "normalization" procedure. In our case, we have calibrated the spin polarization of our electron source to  $P = 29 \pm 3\%$ , see Ref. 12. We demonstrate in Fig. 3, how this uncertainty in  $P$  influences the determination of the conduction-band spin splitting at the  $\bar{K}$  valley of WS<sub>2</sub>. In the left-hand panel, the spin-resolved raw inverse-photoemission data is presented. The additional three panels show the individual spin spectra, derived with Eq. 6 for assumed electron-beam spin-polarization values of 32, 29, and 26%. The spin splitting for  $\theta = 80^\circ$  along  $\bar{\Gamma} - \bar{K}$  varies by  $\pm 2$  meV, for  $\theta = 70^\circ$  along  $\bar{\Gamma} - \bar{K}'$  by  $\pm 3$  meV, both well within the given uncertainty margins.

<sup>1</sup> S. D. Stolwijk, H. Wortelen, A. B. Schmidt, and M. Donath, Rev. Sci. Instrum. **85**, 13306 (2014).

<sup>2</sup> V. Dose and G. Reusing, Appl. Phys. **23**, 131 (1980).

- <sup>3</sup> F. Passek, M. Donath, K. Ertl, and V. Dose, Phys. Rev. Lett. **75**, 2746 (1995).
- <sup>4</sup> F. Passek and M. Donath, Phys. Rev. Lett. **69**, 1101 (1992).
- <sup>5</sup> M. Donath and K. Ertl, Surf. Sci. **262**, L49 (1992).
- <sup>6</sup> J. Kessler, Polarized Electrons, Springer Series on Atoms and Plasmas, 2nd Edition, Vol. 1 (Springer, Berlin, Heidelberg, New York, Tokyo, 1985).
- <sup>7</sup> E. Kisker, “Spin- and angle-resolved photoemission from ferromagnets,” in Polarized Electrons in Surface Physics, edited by R. Feder (World Scientific, Singapore, 1985) Chap. 12, pp. 513–546.
- <sup>8</sup> P. D. Johnson, Rep. Prog. Phys. **60**, 1217 (1997).
- <sup>9</sup> S. D. Stolwijk, A. B. Schmidt, M. Donath, K. Sakamoto, and P. Krüger, Phys. Rev. Lett. **111**, 176402 (2013).
- <sup>10</sup> M. Donath, Appl. Phys. A **49**, 351 (1989).
- <sup>11</sup> M. Donath, Surf. Sci. Rep. **20**, 251 (1994).
- <sup>12</sup> M. Budke, T. Allmers, M. Donath, and G. Rangelov, Rev. Sci. Instrum. **78**, 113909 (2007).
